# Supplementary material for: Unusual transformation of polymer coils in a mixed solvent close to the critical point
Source: arXiv:1805.01003 source file (2018-07-26)
Supplement: Supplementary file 1 [file Supplemental_Material_to_PRL-LS15960.pdf]

*Supplemental Material*

# Unusual transformation of polymer coils in a mixed solvent close to the critical point

Xiong Zheng[1,2], Mikhail A. Anisimov[1,*], Jan V. Sengers[1], and Maogang He[2]

[1]*Institute for Physical Science and Technology and Department of Chemical and Biomolecular Engineering, University of Maryland, College Park, MD 20742, USA*
[2]*Key Laboratory of Thermo-Fluid Science and Engineering, Ministry of Education, Xi'an Jiaotong University, Xi'an, Shaanxi Province, 710049, P.R. China*

*To whom correspondence should be addressed. Email: anisimov@umd.edu.

## 1. Analysis of experimental data

In the main body of the manuscript, we explain the unique choice of our system that exhibits extremely weak critical opalescence. The refractive-index difference between the two components is exceptionally small (~0.002), which makes the critical opalescence detectable only very close to the critical point, when the correlation length significantly exceeds the hydrodynamic radius of a polymer chain. An example of the autocorrelation function $g_2(t)$ obtained very close to the critical point ($\Delta T$=0.04 °C) and the corresponding decay times from a fit to

$$g_2(t) - 1 = \left[ A_1 \exp\left(\Gamma_1 t\right) + A_2 \exp\left(\Gamma_2 t\right)\right]^2, \qquad (1)$$

where $\Gamma_1$ is the rate of the Brownian diffusion of polymer coils, and $\Gamma_2$ is the rate of the diffusive relaxation of the critical fluctuations, are shown in Fig. S1. When the correlation length is of the same order of magnitude as the hydrodynamic radius, it cannot be obtained from the correlation function independently. To obtain reliable data for the hydrodynamic radius in the region where the correlation length and hydrodynamic radius are of the same order, the decay associated with the critical fluctuations ($\Gamma_2$) was fixed at an assigned value known from static light-scattering experiments [1] and from extrapolation of the observed asymptotic power law deduced from our measurements closer to the critical temperature. Since the DLS signal associated with the decay of the critical fluctuations in this region is usually smaller than the signal from the polymer chains, the inclusion of the second decay

does not qualitatively change the results, but it noticeably reduces the experimental uncertainties.

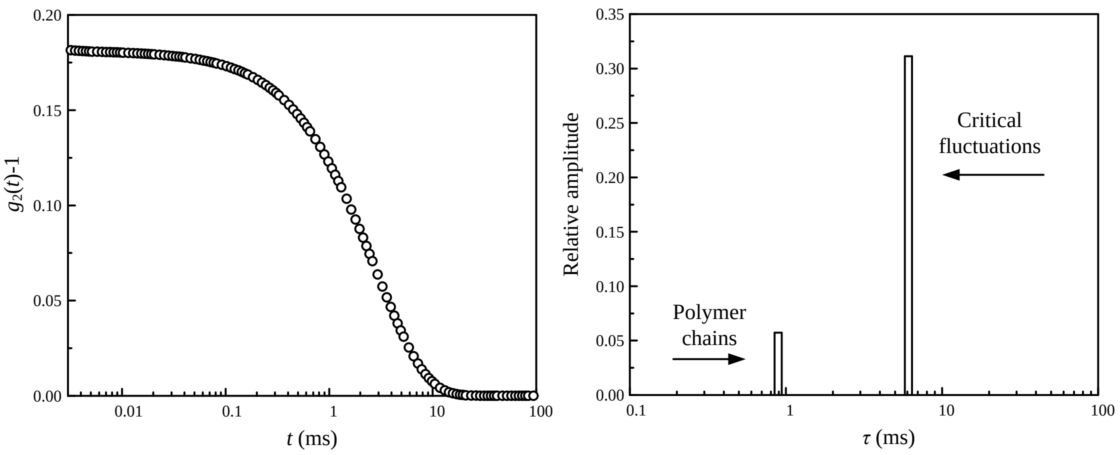


Fig. S1. Correlation function and decay times ($\tau = 1/\Gamma_{1,2}$) for PS-123 at 0.01 % (mass) at Δ$T$=0.04 °C ($T$=30.84 °C).

Fig. S2 shows an example of the correlation function and the decay-time distribution of the critical fluctuations and the polymer chains at Δ$T$=0.15 °C.

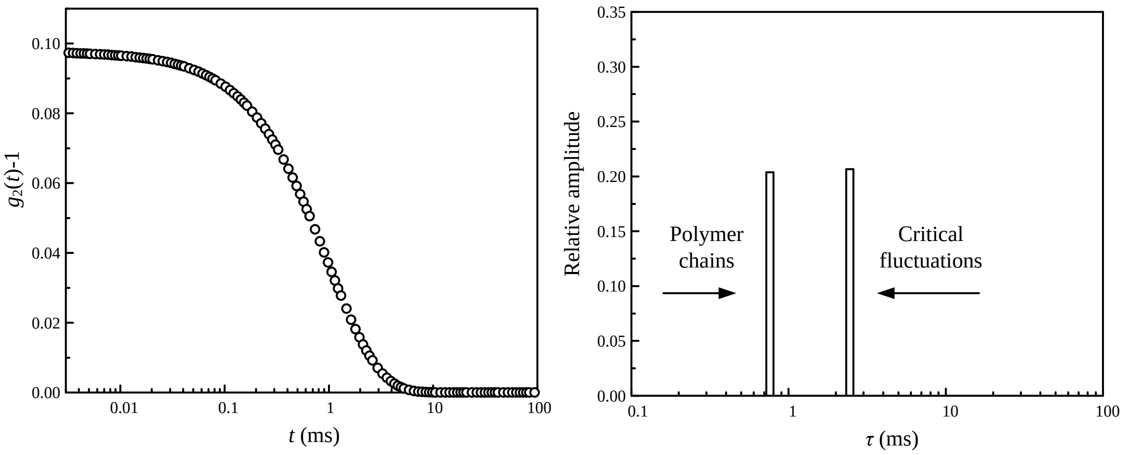


Fig. S2. Correlation function and decay times ($\tau = 1/\Gamma_{1,2}$) for PS-123 at 0.01 % (mass) at Δ$T$=0.15 °C ($T$=30.95 °C).

When the temperature is far away from the critical temperature, the contribution to the DLS correlation function from the critical fluctuations becomes

extremely weak and has no influence on the analysis. Fig. S3 shows the correlation function and the single decay time (attributed to the diffusion of polymer chains) for PS-123 at 0.01 % (mass) when $\Delta T$=5 °C ($T$=35.8 °C).

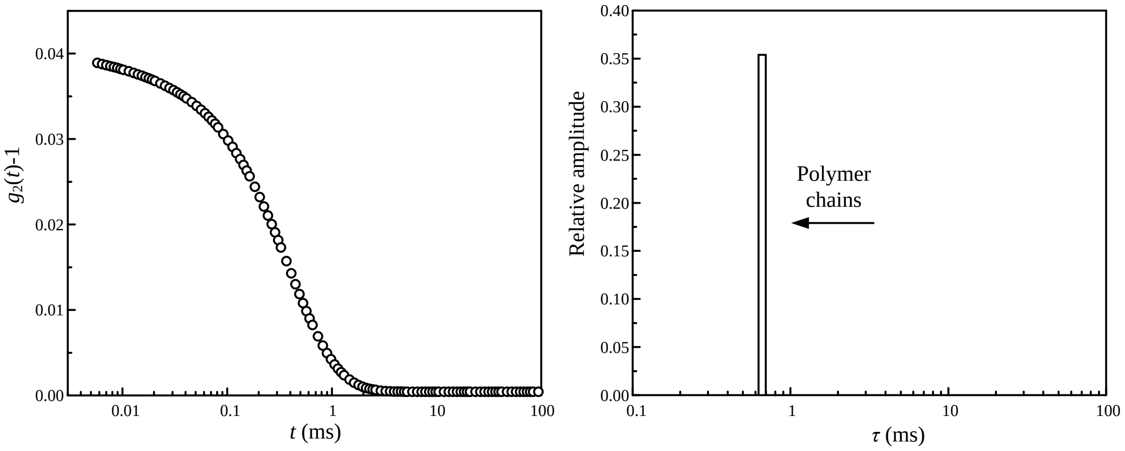


Fig. S3. Correlation function and decay time ($\tau = 1/\Gamma_{1,2}$) (attributed to the diffusion of polymer chains) for PS-123 at 0.01 % (mass) at $\Delta T$=5 °C ($T$=35.8 °C).

## 2. Universal relationship between correlation-length amplitude and polymer concentration

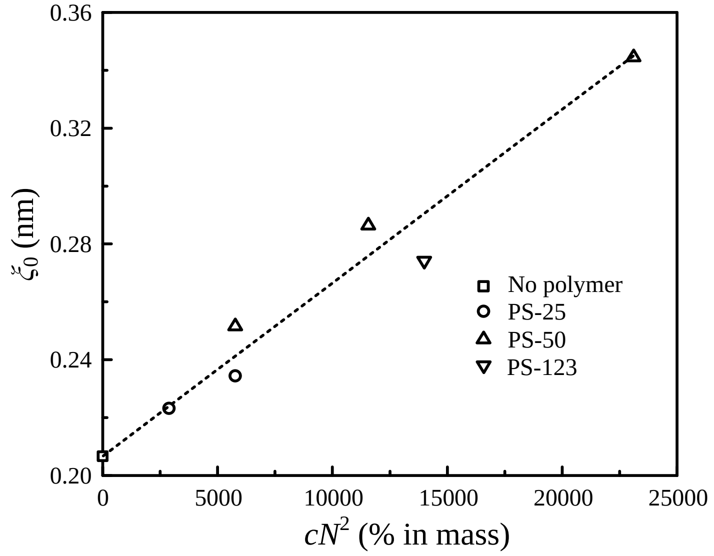


Fig. S4. The amplitude $\xi_0$ follows a universal behavior when the concentration of a polymer is rescaled as $cN^2$.

## 3. Molecular-weight scaling of the hydrodynamic radius of polymer chains and the relationship between hydrodynamic radius and radius of gyration

The exponent *m* in the molecular-weight scaling of the hydrodynamic radius $R_h \propto (M_w)^m$ significantly increases from $m$=0.39 for the collapsed chain to $m$=0.55 for the fully expanded chain.

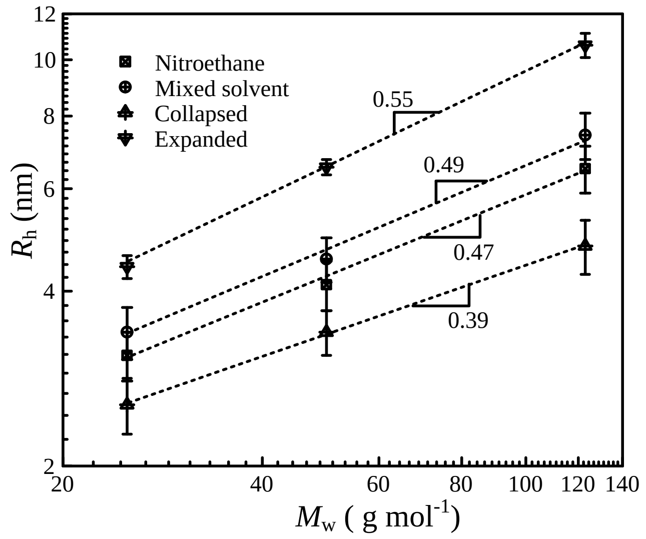


Fig. S5. Molecular-weight scaling of the hydrodynamic radius of polymer chains. The slopes give the value of the exponent *m*.

For a linear polymer chain, the ratio of the radius of gyration $R_g$ and the hydrodynamic radius $R_h$ is related to the solvent quality. When the solvent changes from a good solvent to a theta solvent, $R_g / R_h$ changes from ~ 1.5 to ~ 1.6 [2]. Fig. S5 shows that the hydrodynamic radius of polystyrene in the mixed solvent is slightly higher than that in nitroethane which is close to a theta solvent. It means that the non-ideal mixed solvent is a better solvent for polystyrene than nitroethane, a generic feature predicted by the Shultz and Flory theory [3]. Therefore, it is expected that $R_g / R_h$ of polystyrene chains is between 1.5 and 1.6 in the nitroethane-isooctane

mixture. The fact that the chain collapse begins to be detectable when $\xi \approx R_{\mathrm{h}} \approx 0.6 R_{\mathrm{g}}$ is in full agreement with the explanation of Brochard and de Gennes that the collapse begins when the correlation length becomes of the order of the radius of gyration.

# References

[1] Y. Garrabos, G. Zalczer, and D. Beysens, Phys. Rev. A **25**, 1147 (1982).

[2] I. Teraoka, Polymer Solutions: An Introduction to Physical Properties (Wiley, New York, 2002).

[3] A. R. Shultz and P. J. Flory. J. Polym. Sci. **15**, 231 (1955).
